# Supplementary material for: Summarize and Generate to Back-translate: Unsupervised Translation of Programming Languages
Source: arXiv:2205.11116 source file (2023-02-11)
Supplement: Supplementary file 1 [file 1_error_breakdown.tex]

\begin{table*}[!ht]
\centering
% \resizebox{\linewidth}{!}
{%
% \small%
% \def\arraystretch{1.05}%
\begin{tabular}{l c c}
\hline
Error Category & TransCoder  & PLBART  \\ 
\midrule
\rowcolor{dark-gray}
Total Errors & 149  & 146 \\
\midrule
\rowcolor{light-gray}
Compilation & 0  & 0 \\
\midrule
\rowcolor{light-gray}
Runtime & 149  & 146 \\
\quad AttributeError & 11  & 5 \\
\quad IndexError  & 18  & 20 \\
\quad KeyError  & 3  & 4 \\
\quad NameError  & 17  & 16 \\
\quad OverflowError  & 2  & 1 \\
\quad RecursionError  & 1  & 2 \\
\quad SyntaxError & 26  & 9 \\
\quad TypeError  & 47  & 61 \\
\quad UnboundLocalError & 13  & 11 \\
\quad ValueError  & 11  & 15 \\
\quad ZeroDivisionError & 0  & 2 \\
\hline
\end{tabular}
}
\caption{
% Java to Python (based on greedy search).
Category of errors made by the TransCoder and PLBART models on Java to Python translation (using greedy search). 
}
\label{table:error_analysis_greedy_j_2_p}
% \vspace{-2mm}
\end{table*}

\begin{table*}[!ht]
\centering
% \resizebox{\linewidth}{!}
{%
% \small%
% \def\arraystretch{1.05}%
\begin{tabular}{l c c}
\hline
Error Category & TransCoder & PLBART  \\ 
\midrule
\rowcolor{dark-gray}
Total Errors & 201 & 212 \\
\midrule
\rowcolor{light-gray}
Compilation & 151  & 180 \\
\quad BadOperand  & 15  & 12 \\
\quad CantFindSymbol  & 23  & 30 \\
\quad SyntaxError  & 14  & 25 \\
\quad TypeError  & 89  & 108 \\
\quad Others & 10 & 5 \\
\midrule
\rowcolor{light-gray}
Runtime & 50  & 27 \\
\quad IndexOutOfBoundsException  & 40  & 15 \\
\quad NullPointerException  & 2  & 3 \\
\quad NumberFormatException  & 5  & 6 \\
\quad Others & 3  & 3 \\
\hline
\end{tabular}
}
\caption{
% Python to Java (based on greedy search).
Category of errors made by the TransCoder, and PLBART models on Python to Java translation (using greedy search). 
}
\label{table:error_analysis_p_2_j}
\vspace{-2mm}
\end{table*}
