# Supplementary material for: Summarize and Generate to Back-translate: Unsupervised Translation of Programming Languages
Source: arXiv:2205.11116 source file (2023-02-11)
Supplement: Supplementary file 5 [file 3_model_desc.tex]

% \begin{table}[!tbh]
% \centering
% % \resizebox{\linewidth}{!}
% {%
% % \small%
% % \def\arraystretch{1.05}%
% \begin{tabular}{l c c}
% \hline
%  & TransCoder & PLBART  \\
% \hline
% \#layers* & 6 & 6 \\
% \#heads & 8 & 12 \\
% Model dim & 1024 & 768 \\
% Vocab size & 64,000 & 50,000 \\
% Total parameters  & 312 M & 140 M \\
% \cline{1-3}
% \multicolumn{3}{l}{\textbf{{Stage1: Pre-training}}} \\ 
% \cline{1-3}
% Objective & MLM & DAE \\
% Total tokens & 920 B & 87 B \\
% Token types & BPE & Sentencepiece \\
% \hdashline
% \multirow{3}{*}{Languages} & Java, & Java,\\
% & Python, & Python, \\
% & C++ & English\\
% \hline
% \multicolumn{3}{l}{\textbf{{Stage2: Training}}} \\ 
% \cline{1-3}
% Objective & DAE+BT & BT \\
% Total tokens & 625 M & 430 M \\
% Token types & BPE & Sentencepiece \\
% \hdashline
% \multirow{3}{*}{Languages} & Java, & Java,\\
% & Python, & Python, \\
% & C++ & \\

% \hline
% \end{tabular}
% \\ * \#layers represent both encoder and decoder number of layers.
% }
% \caption{
% Training and parameters setting of Transcoder and out approach.
% }
% \label{table:replication_params}
% % \vspace{-2mm}
% \end{table}

\begin{table*}[!ht]
\centering
% \resizebox{\linewidth}{!}
{%
% \small%
% \def\arraystretch{1.05}%
\begin{tabular}{l c c}
\hline
 & TransCoder & PLBART  \\
\hline
\#layers (encoder) & 6 & 6 \\
\#layers (decoder) & 6 & 6 \\
\#heads & 8 & 12 \\
Model dim & 1024 & 768 \\
Vocab size & 64,000 & 50,000 \\
Total parameters  & 312 M & 140 M \\
\cdashline{1-3}
\multicolumn{3}{l}{{Stage1: Pre-training}} \\ 
\cdashline{1-3}
Objective & MLM & DAE \\
Total tokens & 920 B & 87 B \\
Token types & BPE & Sentencepiece \\
Languages & Java, Python, C++ & Java, Python, English \\
\cdashline{1-3}
\multicolumn{3}{l}{{Stage2: Training}} \\ 
\cdashline{1-3}
Objective & DAE+BT & BT \\
Total tokens & 625 M & 430 M \\
Token types & BPE & Sentencepiece \\
Languages & Java, Python, C++ & Java, Python \\
\hline
\end{tabular}
}
\caption{
TransCoder vs. PLBART.
}
\label{table:replication_params}
% \vspace{-2mm}
\end{table*}

% \begin{table}[!ht]
% \centering
% \resizebox{\linewidth}{!}
% {%
% % \small%
% % \def\arraystretch{1.05}%
% \begin{tabular}{l c@{\hskip 0.1in} c}
% \hline
%  & TransCoder & PLBART  \\
% \hline
% \#Enc-layers & 6 & 6 \\
% \#Dec-layers & 6 & 6 \\
% \#Heads & 8 & 12 \\
% Model dim & 1024 & 768 \\
% Vocab size & 64,000 & 50,000 \\
% Total parameters  & 312 M & 140 M \\
% \cdashline{1-3}
% \multicolumn{3}{l}{{Stage1: Pre-training}} \\ 
% \cdashline{1-3}
% Objective & MLM & DAE \\
% Total tokens & 920 B & 87 B \\
% Token types & BPE & Sentencepiece \\
% Languages & \makecell{Java, Python, \\ C++} & \makecell{Java, Python, \\ English} \\
% \cdashline{1-3}
% \multicolumn{3}{l}{{Stage2: Training}} \\ 
% \cdashline{1-3}
% Objective & DAE+BT & BT \\
% Total tokens & 625 M & 430 M \\
% Token types & BPE & Sentencepiece \\
% Languages & \makecell{Java, Python,\\ C++} & Java, Python \\
% \hline
% \end{tabular}
% }
% \caption{
% TransCoder vs. PLBART.
% }
% \label{table:replication_params}
% % \vspace{-2mm}
% \end{table}
